# Supplementary material for: Adaptive Test Allocation for Outbreak Detection and Tracking in Social Contact Networks
Source: arXiv:2011.01998 source file (2020-11-03)
Supplement: Supplementary file 1 [file ex_supplement.tex]

% SIAM Supplemental File Template
\documentclass[final,supplement,onefignum,onetabnum]{siamart171218}

\input{ex_shared}

%% Use \myexternaldocument on Overleaf
\myexternaldocument{ex_article}

% Optional PDF information

\begin{document}

\maketitle

\bibliographystyle{siamplain}
\bibliography{references}

\end{document}
